# Supplementary material for: Efficient Multi-Instance Generation with Janus-Pro-Dirven Prompt Parsing
Source: arXiv:2503.21069 source file (2025-03-27)
Supplement: Supplementary file 1 [file X_suppl.tex]

\setcounter{figure}{0}
\setcounter{table}{0}

\clearpage
\setcounter{page}{1}
\maketitlesupplementary
\begin{figure}[ht]
\centering
\includegraphics[width=1\linewidth]{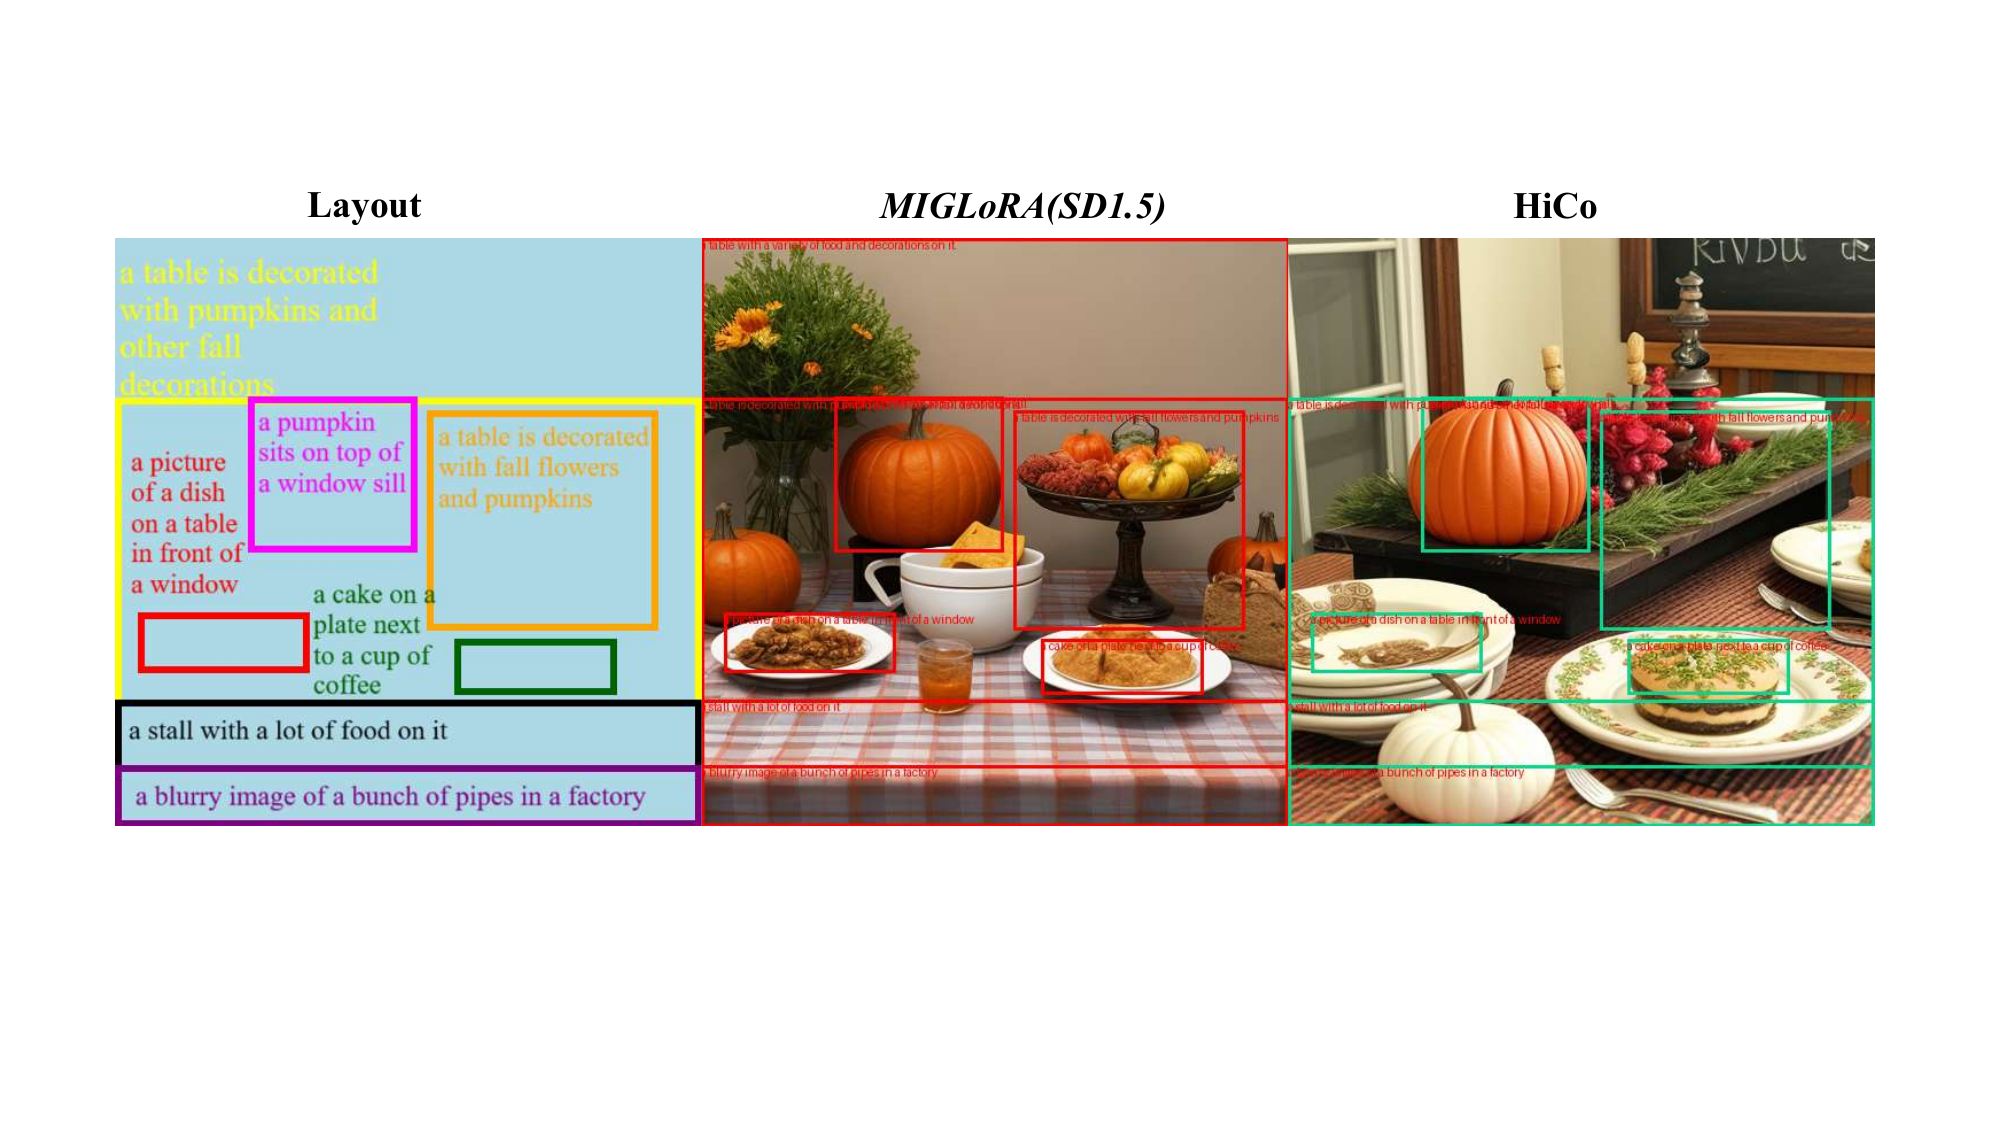} 
\caption{An example tested on COCO Val demonstrates the following: (1) The task requires generating an image of a table filled with food based on specified positional and color attributes; (2) Our proposed \textit{MIGLoRA(SD1.5)} not only generates food and decorations according to the specified positions in the annotations but also ensures that the attributes of each generated instance are accurate; (3) In contrast, the state-of-the-art layout-to-image method HiCo~\cite{37} fails to generate the positions and attributes of instances accurately.
}
\label{fig:head}
\end{figure}

We provide additional details in the supplementary material, and the model is made publicly available upon acceptance of the paper. The supplementary material includes a detailed explanation of the dataset construction (Sec \ref{sec:mig-dataset}), comparison of parameter count(Sec \ref{parameter}), implementation details (Sec \ref{details}), and additional experimental results (Sec \ref{sec:mig-results}\&\ref{D}\&\ref{E}).

\section{Dataset Construction}
\label{sec:mig-dataset}
We construct the DescripBox dataset for training and the DescripBox-Val dataset for testing using essentially the same process.
Unlike standard object detection datasets, our dataset provides highly detailed instance-level prompts for each object in the image, enabling more precise control over the content of generated images. 

\paragraph{Data Collection:}
The processing steps are described as follows:
\begin{itemize}
    \item \textbf{Global Prompt Generation}: To generate a concise description of the overall content of the image, we use the BLIP model. Since detailed descriptions are provided for each object in the image subsequently, the global description does not need to be complex; it only needs to accurately summarize the image content. The BLIP model, which generates brief and precise textual descriptions from image input, is thus selected as the optimal solution.
    
    \item \textbf{Image Segmentation and Mask Generation}: Next, we perform image segmentation and generate the corresponding masks. We utilize the RAM\cite{45} and Grounded-SAM models for this process. The RAM model is an image annotation tool that generates a series of fine-grained labels based on the input image and global prompt, such as \textit{"dog"}, \textit{"woman"}, and \textit{"hand"}. Grounded-SAM\cite{16} is composed of GroundingDino and the Segment Anything Model (SAM)\cite{12}. GroundingDino processes key labels to detect objects related to the prompt in the image and generates corresponding bounding boxes. SAM then takes these bounding boxes as input and produces pixel-level segmentation masks within the specified regions.
    
    \item \textbf{Instance-Level Prompt Generation}: Finally, we use the bounding boxes generated in the previous step to crop the original image and extract the corresponding object regions. For each cropped object region, we use the pre-trained BLIP-V2 model\cite{46} to generate high-quality instance-level textual prompts, such as \textit{"a man in a leather jacket standing in front of a building"}. The BLIP-V2 model integrates visual and linguistic information to accurately describe the appearance, attributes, and contextual details of the objects, thus provides richer and more fine-grained descriptions for subsequent tasks.
\end{itemize}

\paragraph{Image Screening Process:}
Furthermore, we develop a robust scoring system to filter out low-quality images. 
This system evaluates images based on their size, the confidence of bounding boxes, and their absolute and relative positions. It calculates bounding box confidence scores, area penalties, and overlap penalties, ultimately deriving a comprehensive total score. Based on this total score, images with a score of 60 or higher are classified as high-quality, while those scoring below 60 are categorized as low-quality.

The scoring system evaluates image quality based on bounding box confidence, relative size, and overlap penalties. The total score is calculated as follows:

\[
\text{Total Score} = 100 \cdot \left( \frac{C}{N} - \lambda_A \cdot P_A - \lambda_O \cdot P_O \right)
\]
Here, \( C \) is the sum of the confidence scores of all bounding boxes, normalized by the number of bounding boxes \( N \). It is defined as:

\[
C = \sum_{i=1}^{N} c_i
\]
where \( c_i \in (0, 1) \) represents the confidence of the \( i \)-th bounding box. The area penalty \( P_A \) accounts for the relative size of bounding boxes compared to the image area:

\[
P_A = \frac{1}{N} \sum_{i=1}^{N} \frac{A_i}{A_T}
\]
where \( A_i \) is the area of the \( i \)-th bounding box and \( A_T \) is the total area of the image. The overlap penalty \( P_O \) measures the average overlap between pairs of bounding boxes:

\[
P_O = \frac{1}{N(N-1)} \sum_{i=1}^{N} \sum_{j=i+1}^{N} O_{ij}
\]
where \( O_{ij} \in [0, 1] \) is the normalized overlap ratio (e.g., Intersection over Union) between the \( i \)-th and \( j \)-th bounding boxes. The parameters \( \lambda_A \) and \( \lambda_O \) are the weights for the area and overlap penalties, respectively.

Through extensive experimentation and comparisons with manually curated datasets, we identify two critical thresholds: the area penalty weight \( \lambda_A \) is set to 0.3, and the overlap penalty weight \( \lambda_O \) is set to 0.7. These values are chosen to achieve an optimal balance between filtering out low-quality images and retaining high-quality ones.
This scoring system achieves a balanced evaluation by integrating confidence, size, and overlap into a single metric. It enables precise filtering of low-quality images and facilitates the creation of a high-quality dataset.

\begin{figure}[ht]
%\vspace{-10mm}
\centering
\includegraphics[width=0.5\textwidth]{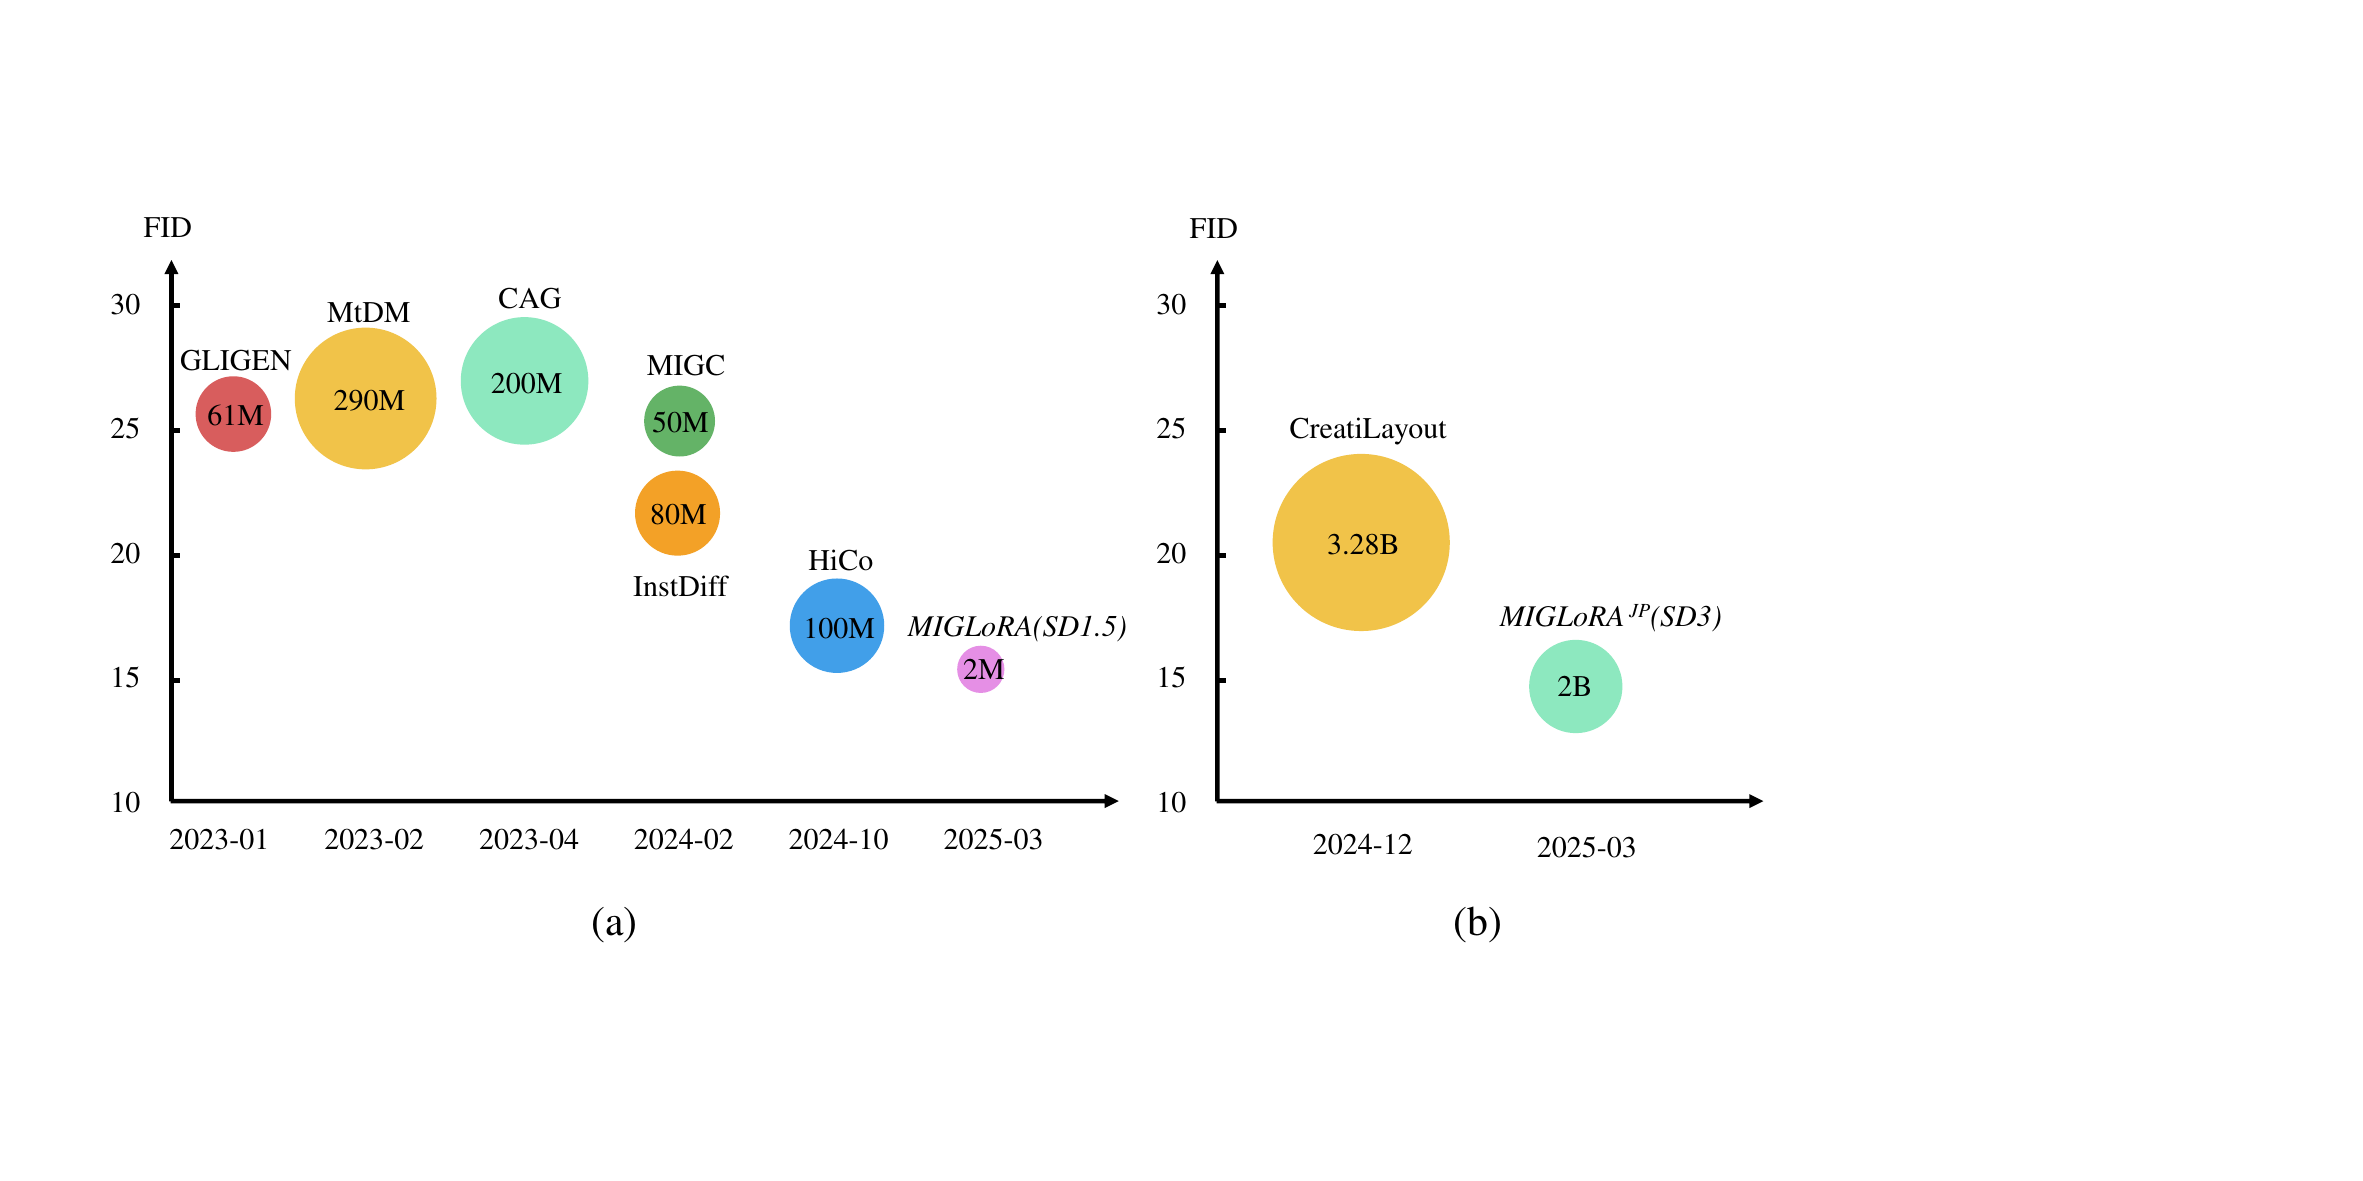} 
\caption{Comparison of the number of parameters between SOTA and our method: (a) models based on SD1.5, (b) models based on SD3.}
\label{fig:parameters}
\end{figure}

\section{Comparison of Parameters}
\label{parameter}
As shown in Figure~\ref{fig:parameters}, we compare the number of parameters of current SOTA methods with our proposed approach. Among models using SD1.5 as the backbone, our method significantly reduces parameters compared to other models while maintaining excellent performance. For models based on SD3, our approach reduces parameters by 47\% compared to CreatiLayout while achieving substantially better performance.

%\paragraph{Low Rank Adaption}
%For our LoRA fine-tuning approach, we decompose the weight updates into low-rank transformations:
%\begin{equation}
%W = W_{0} + BA \label{eq:lora}
%\end{equation}
%where $W_{0}$ represents the original pre-trained weights that remain frozen, while $B \in \mathbb{R}^{d \times r}$ and $A \in \mathbb{R}^{r \times d}$ are trainable low-rank matrices with rank $r$. This approach significantly reduces the number of trainable parameters while maintaining model performance.

\section{More Implementation Details}
\label{details}
\textbf{Training:} We train our \textit{MIGLoRA(SD1.5)} model on the \textit{DescripBox} dataset, employing a learning rate of $1 \times 10^{-4}$ and the AdamW~\cite{51} optimizer with $\beta_1 = 0.9$, $\beta_2 = 0.999$, weight decay of $1 \times 10^{-2}$, and $\epsilon = 1 \times 10^{-8}$. The model is trained for 40K iterations with a batch size of 256 and a resolution of $512 \times 512$, applying gradient accumulation over 2 steps to improve computational efficiency. Checkpoints are saved every 25,000 steps, with a constant learning rate scheduler applied. Gradient clipping, with a maximum norm of 1.0, is applied to ensure stability, and mixed precision training (FP16) is used, with a noise offset of 0.02 to enhance diffusion regularization. A fixed seed of 42 ensures reproducibility. The entire training process is conducted on 16 NVIDIA H100 GPUs. \textit{MIGLoRA(SD1.5)} is based on Stable Diffusion 1.5, utilizing LoRA~\cite{49} fine-tuning to optimize the linear layers of the UNet~\cite{50}. This configuration significantly enhances the model's performance and stability in the diffusion process.
\textbf{Inference:} We use the UniPCMultistepScheduler to optimize the diffusion process with 50 sampling steps and apply the mask encoder during the first 25 steps. The CFG scale is set to 7.5. As detailed in the implementation, the bounding box information for each object instance is processed via the \texttt{calculate\_weights} function to compute normalized weights inversely proportional to the bounding box area, ensuring effective attention distribution. During inference, the number of instances $n_{\text{infer}}$ is dynamically padded to the maximum number of instances, $n_{\text{max}}$ with zero-filled masks. 

%To construct the conditioning input for the model, each instance's bounding box is converted into binary masks $f_{\text{mask}} \in \mathbb{R}^{1, C, H, W}$, where $C$ denotes the color channels, and $H, W$ are the spatial dimensions. The masks are then stacked into a tensor $f_{\text{cond}} \in \mathbb{R}^{n_{\text{infer}}, H, W}$ and processed through the mask encoder to extract feature embeddings $f_{\text{encoded}} \in \mathbb{R}^{n_{\text{infer}}, d}$, where $d$ is the latent dimensionality. For instances fewer than $n_{\text{max}}$, the additional padding is achieved via duplicate zero-feature masks to form a complete tensor $f \in \mathbb{R}^{n_{\text{max}}, d}$.

%For randomization during training, the instance ordering within $f_{\text{encoded}}$ is shuffled to improve robustness, excluding the background and template shading elements. Guidance scale and inference steps are dynamically adjusted based on input requirements, ensuring efficient computational complexity. The final processed feature embeddings and bounding box information are provided to the Stable Diffusion LoRAMultiLayoutPipeline for generation. During training, bounding box features and mask embeddings are jointly optimized to reduce redundancy and enable high-quality multi-instance attention for shading inference.

\begin{table}
\setlength\tabcolsep{1 pt}
\centering
\small
\begin{tabular}{lcccccccc}
\toprule       
\textbf{Method}  & \textbf{position$\uparrow$} &  \textbf{clarity$\uparrow$}  & \textbf{rationality$\uparrow$} &\textbf{aesthete$\uparrow$} \\
\midrule
MtDM\cite{11}                 & 4.32             &  5.61         &   4.55       &  4.31           \\
GLIGEN\cite{34}               & 7.56            &   5.79        &   5.12        &  4.99         \\
CAG\cite{14}                  &  5.25            &  5.35         &   5.08        &  4.76           \\
MIGC\cite{33}                 & 6.33             &  5.55         &  4.83         &  4.64           \\
HiCo\cite{37}                 &  \cellcolor[HTML]{b1f49e}8.46             &  \cellcolor[HTML]{b1f49e}7.23         &   \cellcolor[HTML]{b1f49e}5.44        &  \cellcolor[HTML]{b1f49e}5.50           \\
InstDiff\cite{36}             & 7.89             &  6.52         &  5.30         &  5.16           \\
\midrule
\textit{MIGLoRA}&  \cellcolor[HTML]{a4c1f7}8.87&\cellcolor[HTML]{a4c1f7}8.01    & \cellcolor[HTML]{a4c1f7}5.68    & \cellcolor[HTML]{a4c1f7}5.69\\
\bottomrule
\end{tabular}
\caption{Quantitative comparison of various methods on the COCO Val dataset for manual evaluation. The metrics include position accuracy, clarity, rationality, and aesthetic appeal, rated by human evaluators to assess the performance of multi-instance generation methods.}
\label{manual}
\end{table}
%\vspace{-5mm}

\section{More Qualitative Results}
\label{sec:mig-results}
Additional qualitative results on the DescripBox-Val dataset are presented in Figure \ref{fig:sd3}. Our method demonstrates superior performance in addressing complex scenarios. Compared to prior SOTA methods, \textit{MIGLoRA} achieves more precise control over object positioning, attribute consistency, and quantity management. This underscores the effectiveness and robustness of our approach in tackling the challenges inherent to multi-model and conditional generation tasks.

\begin{figure*}[ht]
%\vspace{-10mm}
\centering
\includegraphics[width=1\textwidth]{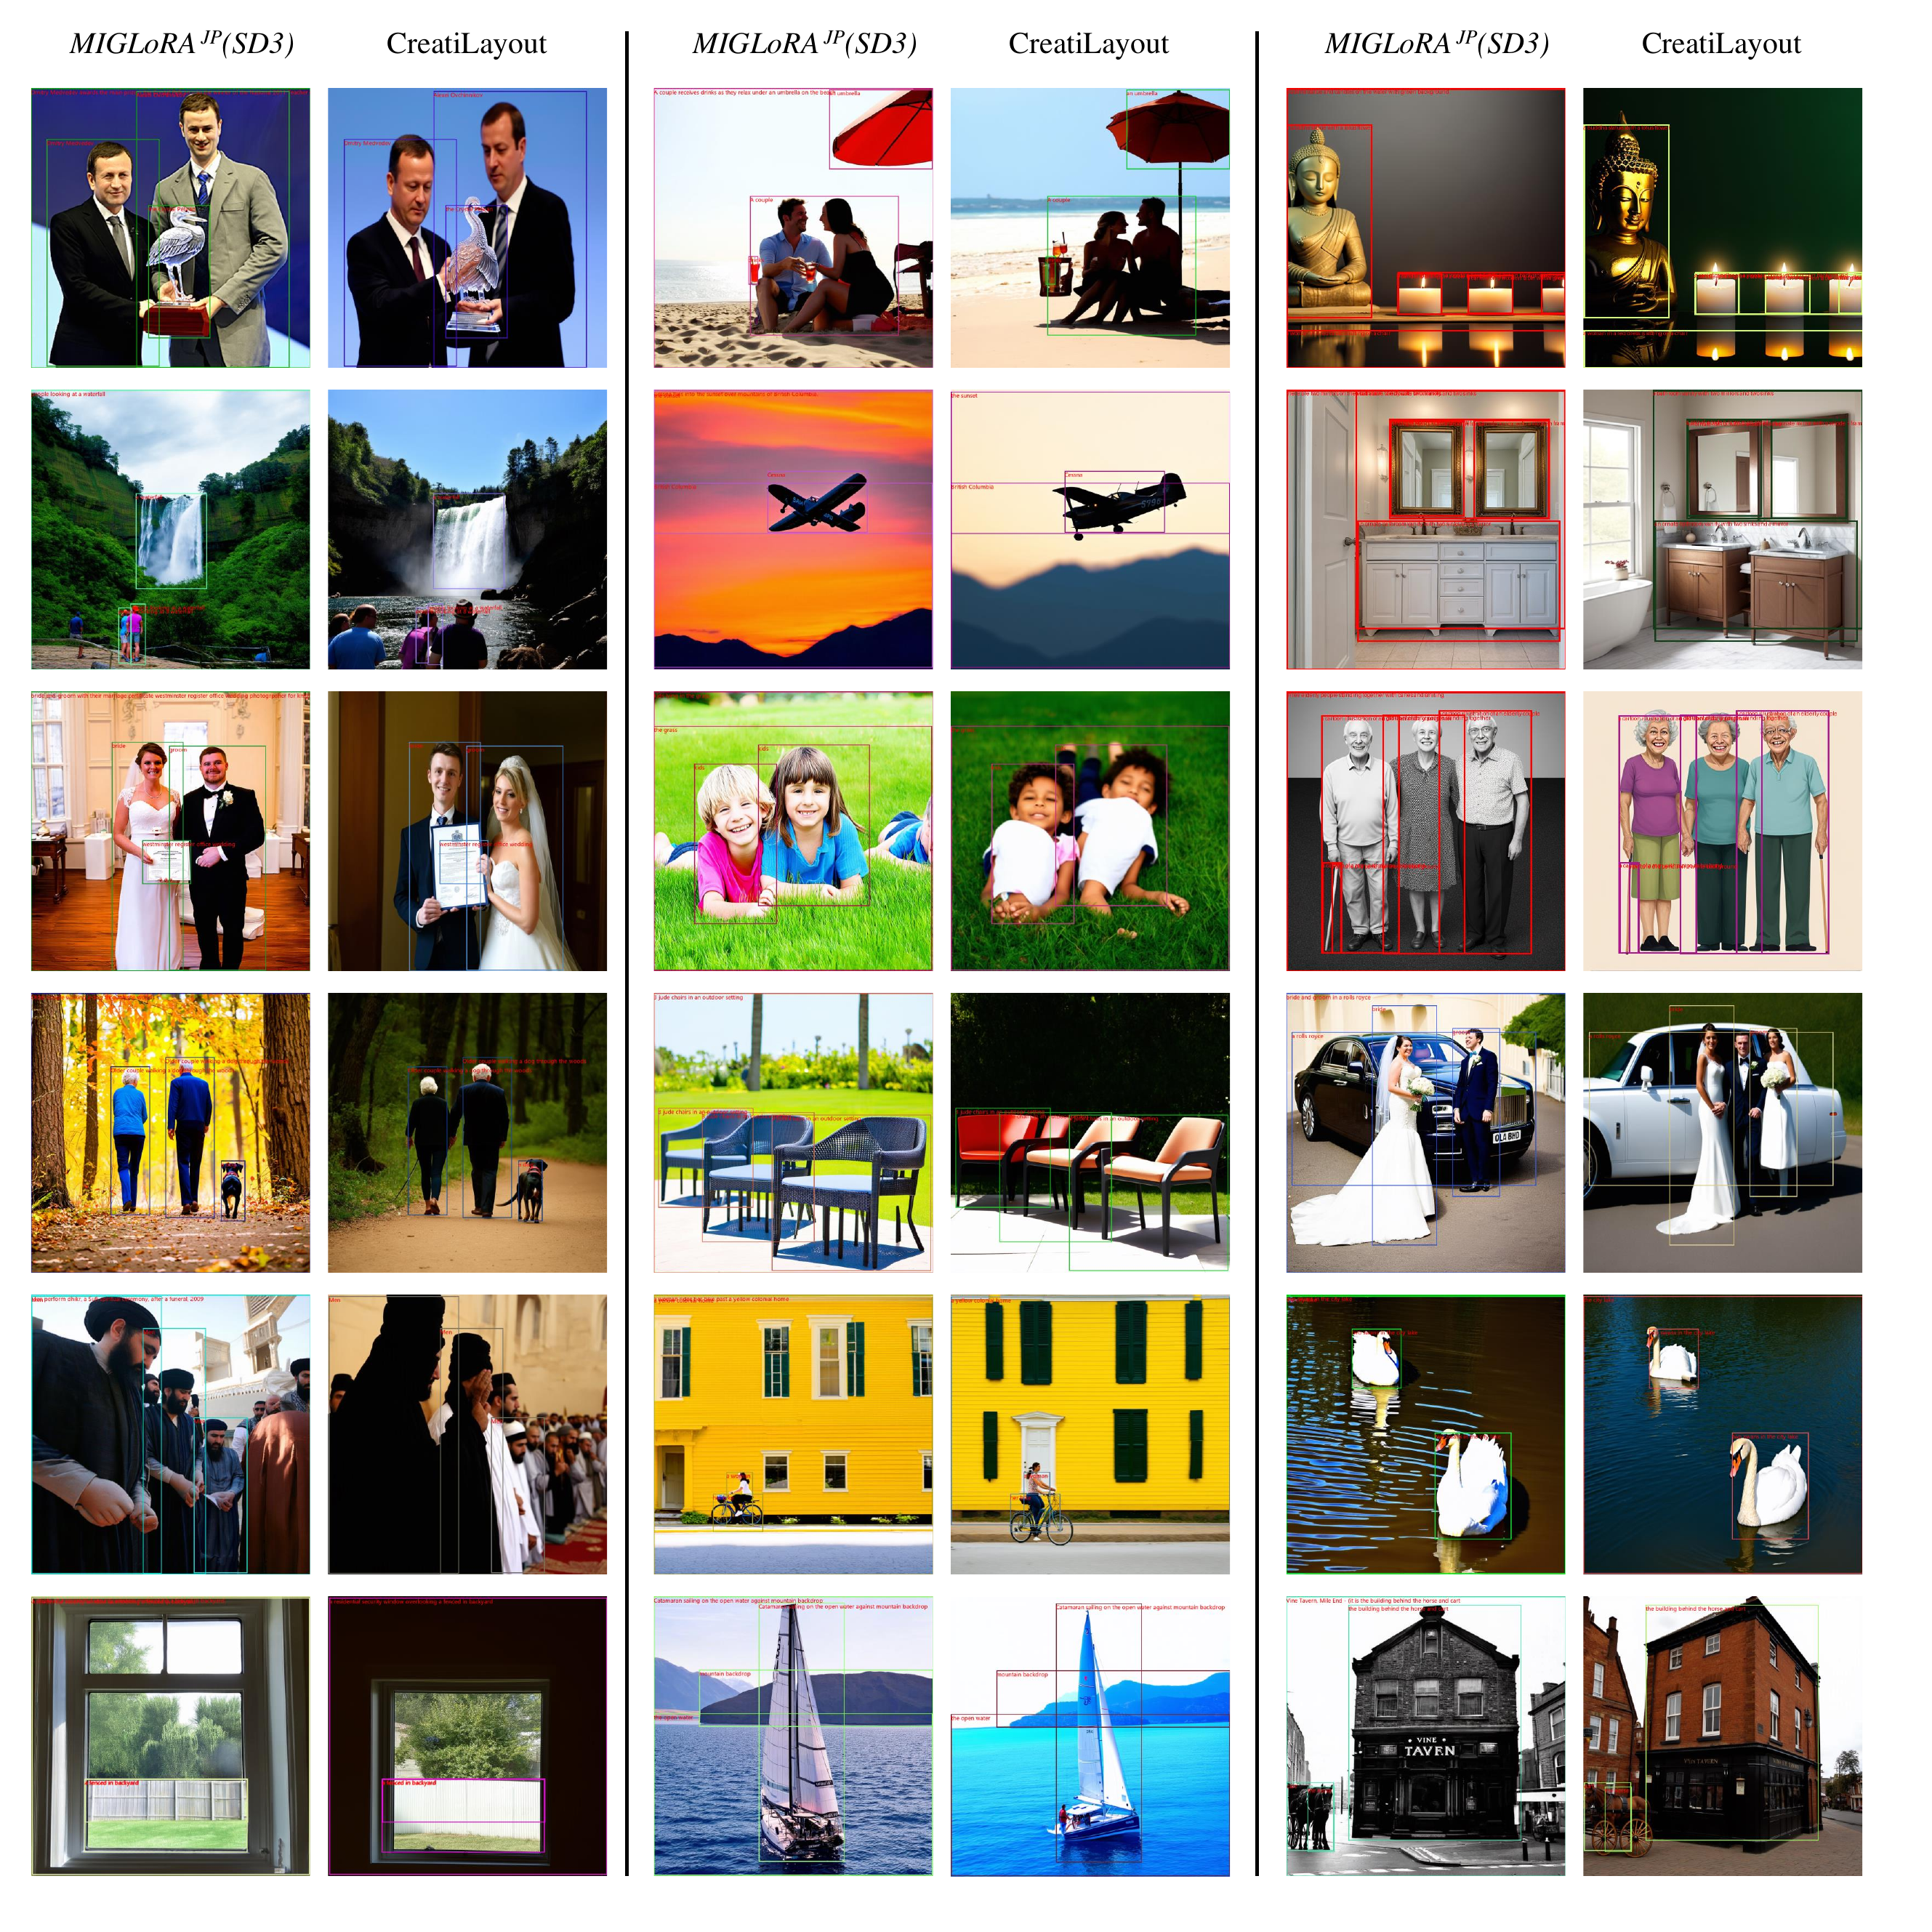} 
\caption{Supplementary qualitative results on the DescripBox-Val dataset. Compared with CreatiLayout, \textit{MIGLoRA\textsuperscript{JP}(SD3)} demonstrates better performance in terms of semantic understanding and object generation accuracy.}
\label{fig:sd3}
%\vspace{10mm}
\end{figure*}

\section{Precise Multi-Instance Generation}
\label{D}
Figures \ref{fig:sd1.5_multi_object} and \ref{fig:SD1.5_control} present additional results obtained using \textit{MIGLoRA} for multi-instance generation. Even with complex layouts and detailed attribute descriptions, \textit{MIGLoRA} ensures that each instance is generated in the correct position with accurate attributes. Furthermore, when the attributes of instances are modified, the model can accurately generate images with the updated attributes while preserving the original image layout as closely as possible.

\begin{figure*}[ht]
%\vspace{-10mm}
\centering
\includegraphics[width=1\textwidth]{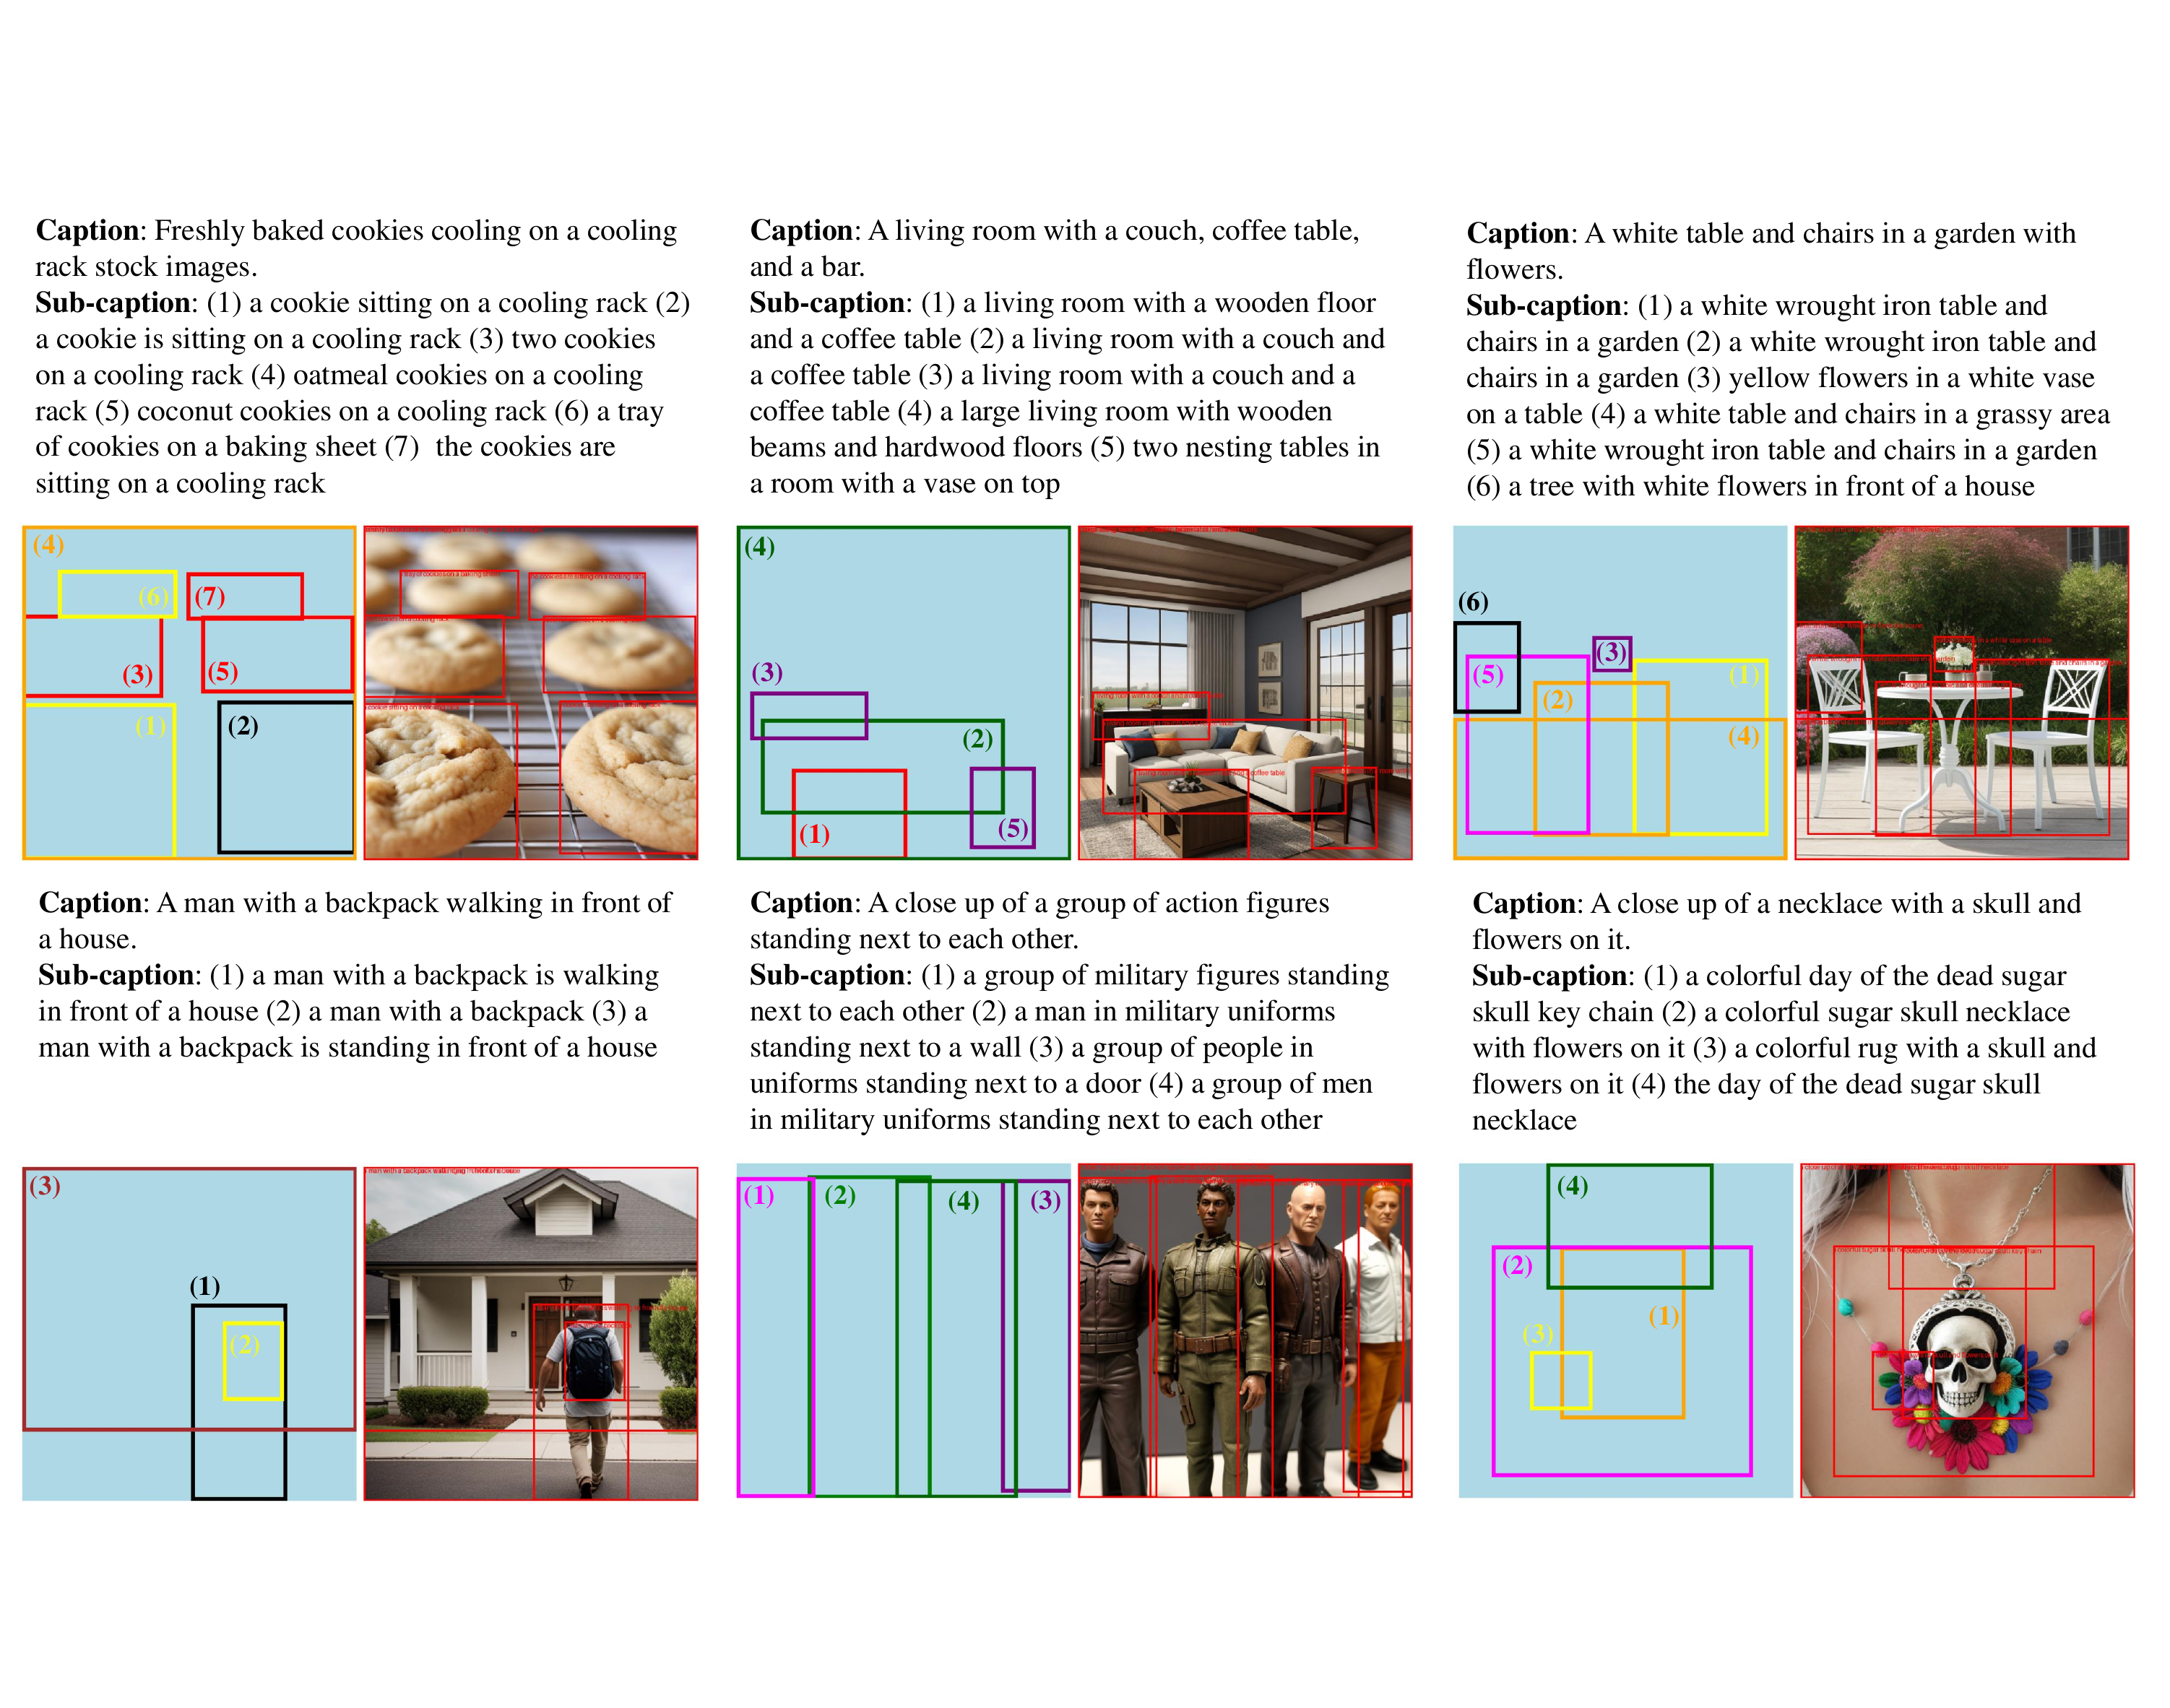} 
\caption{\textit{MIGLoRA\textsuperscript{JP}(SD3)} demonstrates superior performance in complex scenarios and effectively handles multiple bounding boxes while maintaining high-quality outputs. This highlights the model's ability to process detailed and complex visual representations with precision and consistency.}
\label{fig:sd1.5_multi_object}
\end{figure*}

\begin{figure*}[ht]
\centering
\includegraphics[width=0.95\textwidth]{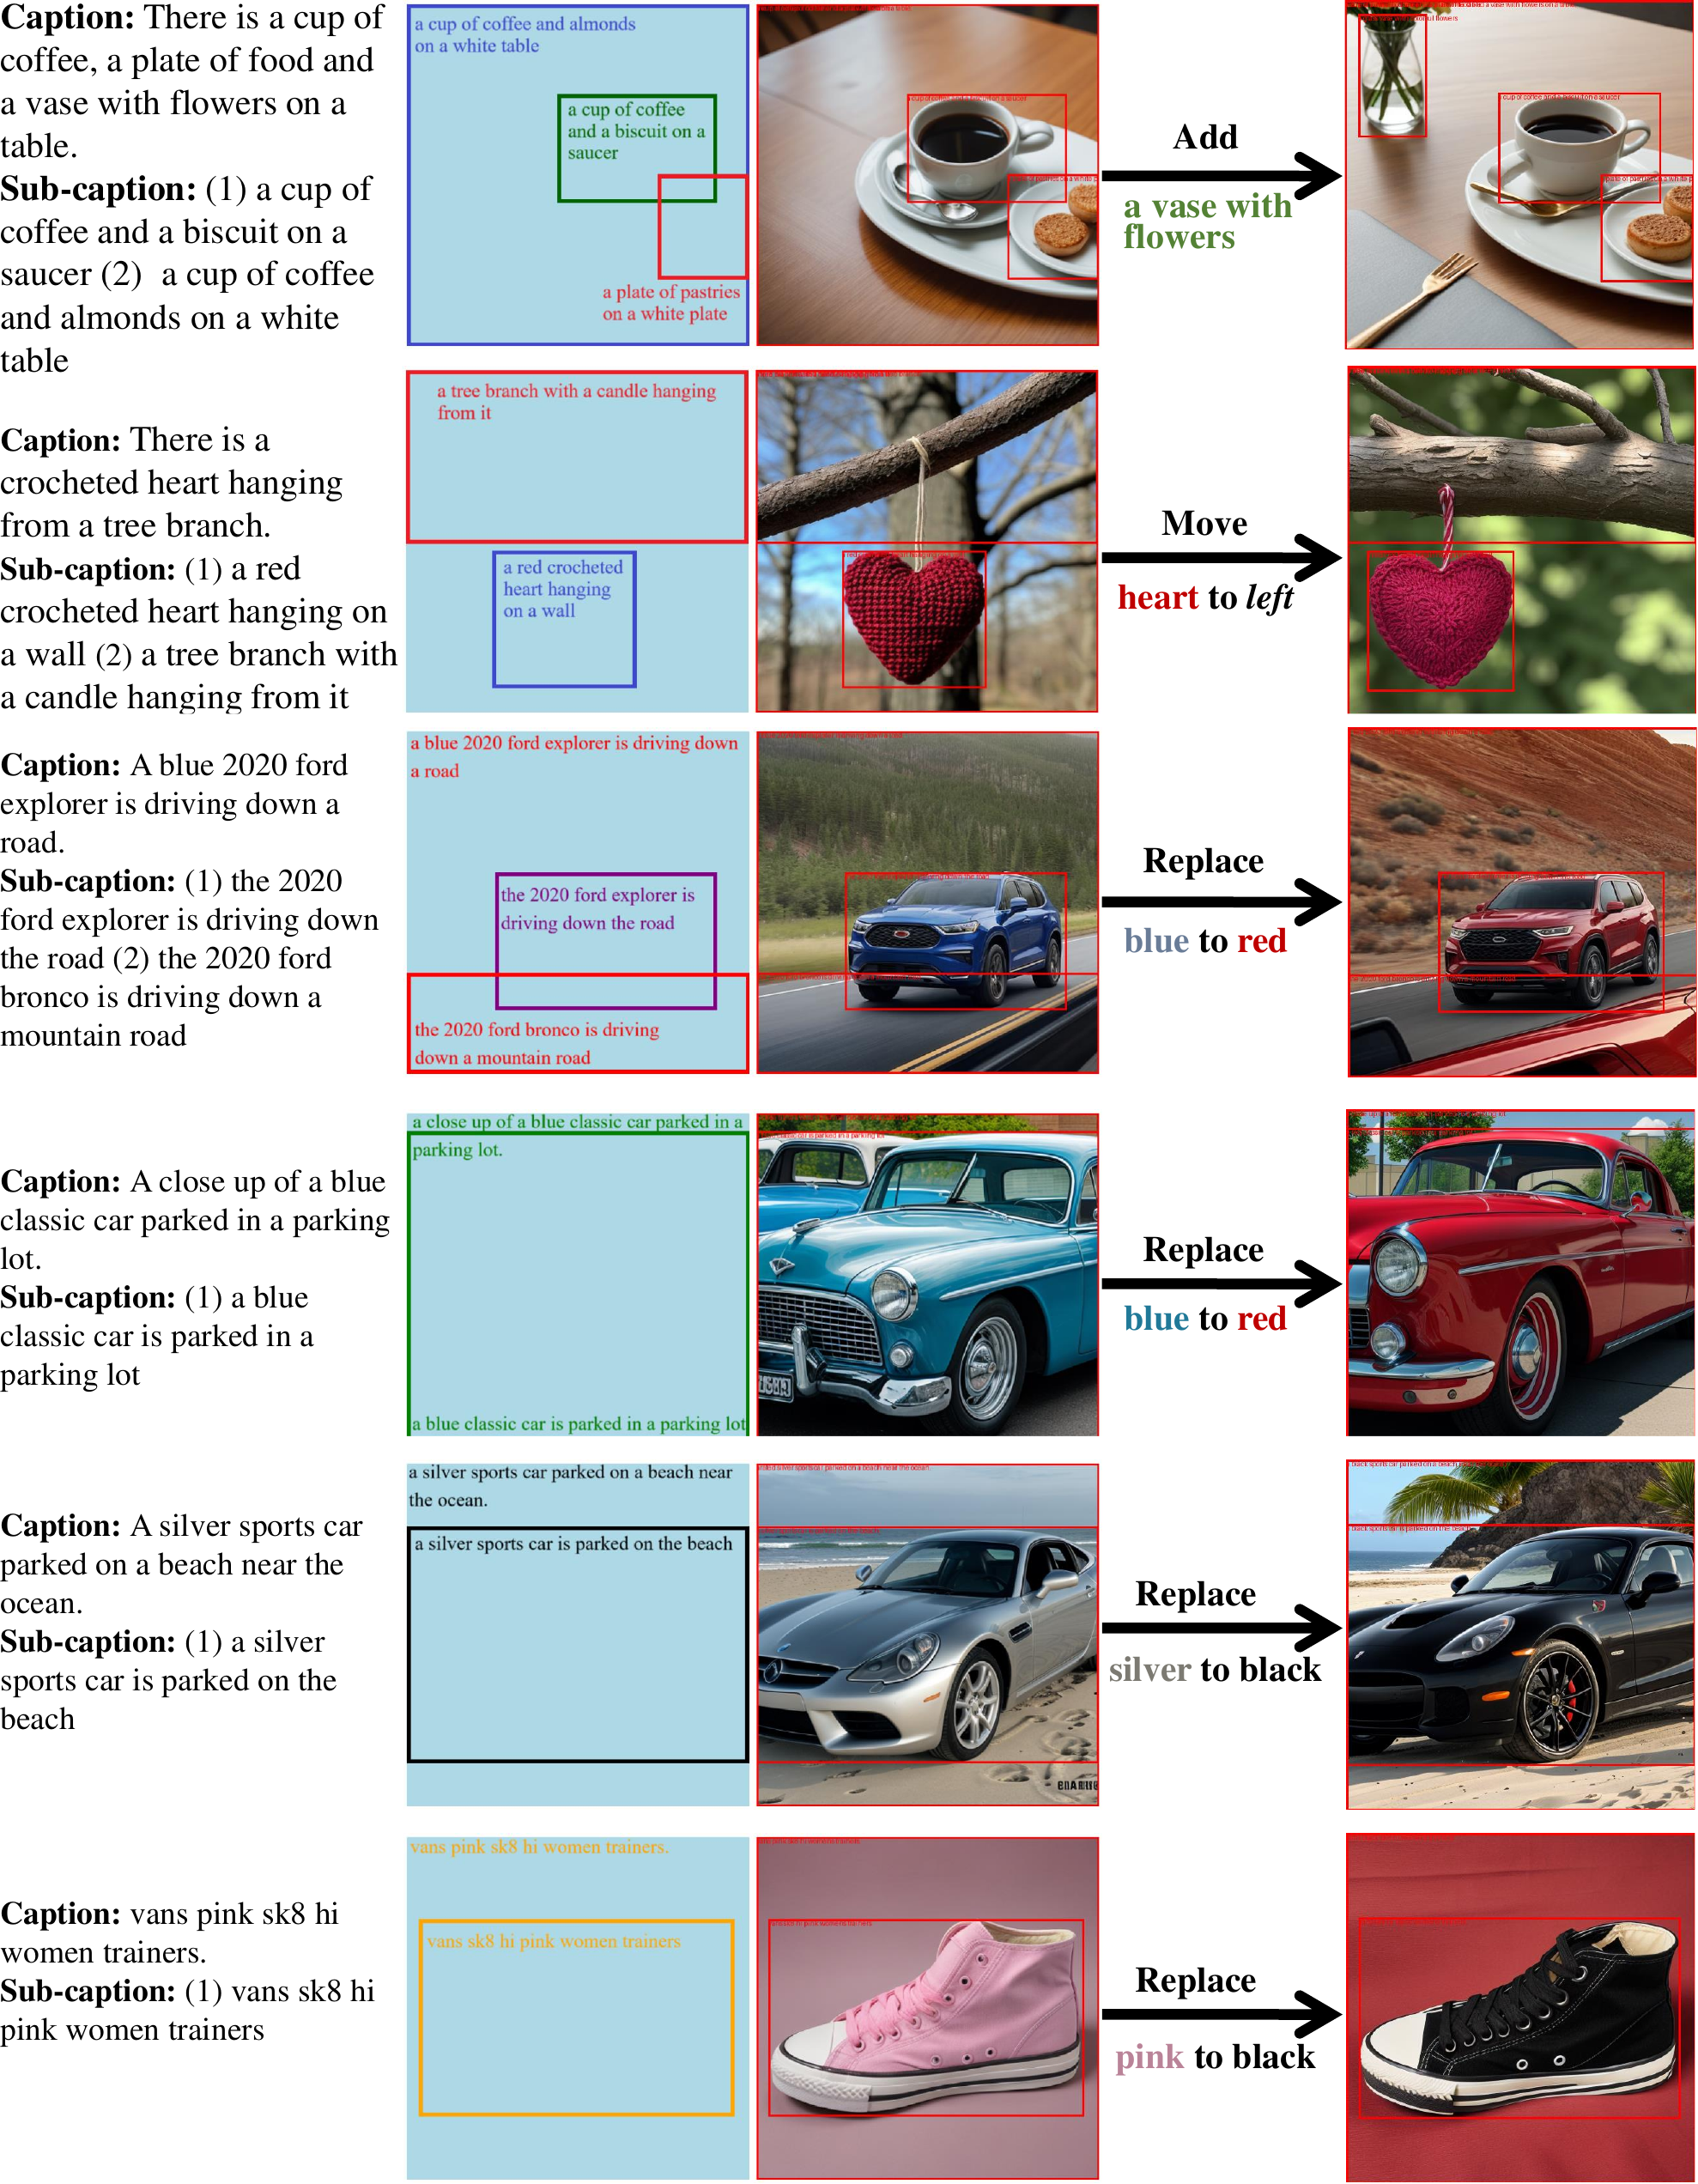} 
\caption{\textit{MIGLoRA\textsuperscript{JP}(SD1.5)} demonstrates strong controllability across diverse scenarios, enabling targeted modifications and the generation of desired scenes or objects through adjustments of descriptive attributes, including contextual changes, object relocation, and color replacement. These results highlight the model's robustness and flexibility in handling complex tasks.}
\label{fig:SD1.5_control}
\end{figure*}

\section{Manual Evaluation on COCO Val}
\label{E}
As shown in Table \ref{manual}, we also conduct a manual evaluation of MIGLoRA to assess the position and clarity of the generated images, alongside scoring their aesthetics and rationality.
Specifically, ten participants rate the generated images across four dimensions: position accuracy, clarity of the depicted elements, rationality of the overall scene composition, and aesthetic appeal. 
The evaluation is performed on the COCO Val dataset to ensure fairness and consistency in benchmarking.
For comparison, we include several baseline methods: MtDM~\cite{11}, GLIGEN~\cite{34}, CAG~\cite{14}, MIGC~\cite{33}, HiCo~\cite{37}, and InstDiff~\cite{36}.
The results demonstrate the superiority of our approach in maintaining positional accuracy and visual coherence, as reflected in the higher scores across all categories.

\begin{figure*}[ht]
\centering
\includegraphics[width=1\textwidth]{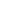} 
\caption{Supplementary qualitative results on the COCO Val dataset, highlighting the performance of \textit{MIGLoRA(SD1.5)} in handling complex scenarios with enhanced control over object positioning, attribute consistency, and quantity management, compared to prior state-of-the-art methods.}
\label{fig:sd1.5_10*7}
\vspace{10mm}
\end{figure*}
